# Supplementary material for: Local Implicit Grid Representations for 3D Scenes
Source: arXiv:2003.08981 source file (2020-03-19)
Supplement: Supplementary file 1 [file arch.tex]

\makeatletter
% Standard Values for Parameters
\newcommand{\tikzcuboid@shiftx}{0}
\newcommand{\tikzcuboid@shifty}{0}
\newcommand{\tikzcuboid@dimx}{4}
\newcommand{\tikzcuboid@dimy}{4}
\newcommand{\tikzcuboid@dimz}{4}
\newcommand{\tikzcuboid@scale}{1}
\newcommand{\tikzcuboid@densityx}{1}
\newcommand{\tikzcuboid@densityy}{1}
\newcommand{\tikzcuboid@densityz}{1}
\newcommand{\tikzcuboid@rotation}{0}
\newcommand{\tikzcuboid@anglex}{0}
\newcommand{\tikzcuboid@angley}{90}
\newcommand{\tikzcuboid@anglez}{225}
\newcommand{\tikzcuboid@scalex}{1}
\newcommand{\tikzcuboid@scaley}{1}
\newcommand{\tikzcuboid@scalez}{1}
\newcommand{\tikzcuboid@linefront}{}
\newcommand{\tikzcuboid@linetop}{}
\newcommand{\tikzcuboid@lineright}{}
\newcommand{\tikzcuboid@fillfront}{}
\newcommand{\tikzcuboid@filltop}{}
\newcommand{\tikzcuboid@fillright}{}
\newcommand{\tikzcuboid@newcoords}{N}
\newcommand{\tikzcuboid@filled}{N}
\newcommand{\tikzcuboid@shaded}{N}
% Definition of Keys
\define@key{tikzcuboid}{shiftx}[\tikzcuboid@shiftx]{\renewcommand{\tikzcuboid@shiftx}{#1}}
\define@key{tikzcuboid}{shifty}[\tikzcuboid@shifty]{\renewcommand{\tikzcuboid@shifty}{#1}}
\define@key{tikzcuboid}{dimx}[\tikzcuboid@dimx]{\renewcommand{\tikzcuboid@dimx}{#1}}
\define@key{tikzcuboid}{dimy}[\tikzcuboid@dimy]{\renewcommand{\tikzcuboid@dimy}{#1}}
\define@key{tikzcuboid}{dimz}[\tikzcuboid@dimz]{\renewcommand{\tikzcuboid@dimz}{#1}}
\define@key{tikzcuboid}{scale}[\tikzcuboid@scale]{\renewcommand{\tikzcuboid@scale}{#1}}
\define@key{tikzcuboid}{densityx}[\tikzcuboid@densityx]{\renewcommand{\tikzcuboid@densityx}{#1}}
\define@key{tikzcuboid}{densityy}[\tikzcuboid@densityy]{\renewcommand{\tikzcuboid@densityy}{#1}}
\define@key{tikzcuboid}{densityz}[\tikzcuboid@densityz]{\renewcommand{\tikzcuboid@densityz}{#1}}
\define@key{tikzcuboid}{rotation}[\tikzcuboid@rotation]{\renewcommand{\tikzcuboid@rotation}{#1}}
\define@key{tikzcuboid}{anglex}[\tikzcuboid@anglex]{\renewcommand{\tikzcuboid@anglex}{#1}}
\define@key{tikzcuboid}{angley}[\tikzcuboid@angley]{\renewcommand{\tikzcuboid@angley}{#1}}
\define@key{tikzcuboid}{anglez}[\tikzcuboid@anglez]{\renewcommand{\tikzcuboid@anglez}{#1}}
\define@key{tikzcuboid}{scalex}[\tikzcuboid@scalex]{\renewcommand{\tikzcuboid@scalex}{#1}}
\define@key{tikzcuboid}{scaley}[\tikzcuboid@scaley]{\renewcommand{\tikzcuboid@scaley}{#1}}
\define@key{tikzcuboid}{scalez}[\tikzcuboid@scalez]{\renewcommand{\tikzcuboid@scalez}{#1}}
\define@key{tikzcuboid}{linefront}[\tikzcuboid@linefront]{\renewcommand{\tikzcuboid@linefront}{#1}}
\define@key{tikzcuboid}{linetop}[\tikzcuboid@linetop]{\renewcommand{\tikzcuboid@linetop}{#1}}
\define@key{tikzcuboid}{lineright}[\tikzcuboid@lineright]{\renewcommand{\tikzcuboid@lineright}{#1}}
\define@key{tikzcuboid}{fillfront}[\tikzcuboid@fillfront]{\renewcommand{\tikzcuboid@fillfront}{#1}}
\define@key{tikzcuboid}{filltop}[\tikzcuboid@filltop]{\renewcommand{\tikzcuboid@filltop}{#1}}
\define@key{tikzcuboid}{fillright}[\tikzcuboid@fillright]{\renewcommand{\tikzcuboid@fillright}{#1}}
\define@key{tikzcuboid}{newcoords}[\tikzcuboid@newcoords]{\renewcommand{\tikzcuboid@newcoords}{#1}}
\define@key{tikzcuboid}{filled}[\tikzcuboid@filled]{\renewcommand{\tikzcuboid@filled}{#1}}
\define@key{tikzcuboid}{shaded}[\tikzcuboid@shaded]{\renewcommand{\tikzcuboid@shaded}{#1}}
% Commands
\newcommand{\tikzcuboid}[1]{
    \setkeys{tikzcuboid}{#1} % Process Keys passed to command
    \begin{scope}[xshift=\tikzcuboid@shiftx,yshift=\tikzcuboid@shifty,scale=\tikzcuboid@scale,rotate=\tikzcuboid@rotation]
    \pgfmathsetmacro{\steppingx}{1/\tikzcuboid@densityx}
    \pgfmathsetmacro{\steppingy}{1/\tikzcuboid@densityy}
    \pgfmathsetmacro{\steppingz}{1/\tikzcuboid@densityz}
    \newcommand{\dimx}{\tikzcuboid@dimx}
    \newcommand{\dimy}{\tikzcuboid@dimy}
    \newcommand{\dimz}{\tikzcuboid@dimz}
    \pgfmathsetmacro{\secondx}{2*\steppingx}
    \pgfmathsetmacro{\secondy}{2*\steppingy}
    \pgfmathsetmacro{\secondz}{2*\steppingz}
    \foreach \x in {\steppingx,\secondx,...,\dimx}
    {   \foreach \y in {\steppingy,\secondy,...,\dimy}
        {   \pgfmathsetmacro{\lowx}{(\x-\steppingx)}
            \pgfmathsetmacro{\lowy}{(\y-\steppingy)}
            \filldraw[fill=orange,draw=blue] (\lowx,\lowy,\dimz) -- (\lowx,\y,\dimz) -- (\x,\y,\dimz) -- (\x,\lowy,\dimz) -- cycle;

        }
    }
    \foreach \x in {\steppingx,\secondx,...,\dimx}
    {   \foreach \z in {\steppingz,\secondz,...,\dimz}
        {   \pgfmathsetmacro{\lowx}{(\x-\steppingx)}
            \pgfmathsetmacro{\lowz}{(\z-\steppingz)}
            \filldraw[fill=green,draw=red] (\lowx,\dimy,\lowz) -- (\lowx,\dimy,\z) -- (\x,\dimy,\z) -- (\x,\dimy,\lowz) -- cycle;
        }
    }
    \foreach \y in {\steppingy,\secondy,...,\dimy}
    {   \foreach \z in {\steppingz,\secondz,...,\dimz}
        {   \pgfmathsetmacro{\lowy}{(\y-\steppingy)}
            \pgfmathsetmacro{\lowz}{(\z-\steppingz)}
            \filldraw[fill=red!50!blue,draw=yellow] (\dimx,\lowy,\lowz) -- (\dimx,\lowy,\z) -- (\dimx,\y,\z) -- (\dimx,\y,\lowz) -- cycle;
        }
    }
    \end{scope}
}

\makeatother

% \begin{document}

% \begin{tikzpicture}
%     \tikzcuboid{shiftx=0cm,%
%         shifty=0cm,%
%         scale=1.00,%
%         rotation=30,%
%         densityx=1,%
%         densityy=2,%
%         densityz=3%
%     }
%     \tikzcuboid{%
%         shiftx=0cm,%
%         shifty=8cm,%
%         scale=1.00,%
%         rotation=60,%
%         densityx=3,%
%         densityy=2,%
%         densityz=5%
%     }
%     \tikzcuboid{%
%         shiftx=8cm,%
%         shifty=8cm,%
%         scale=1.00,%
%         rotation=45,%
%         densityx=0.5,%
%         densityy=1,%
%         densityz=2%
%     }
%     \tikzcuboid{%
%         shiftx=8cm,%
%         shifty=0cm,%
%         scale=1.00,%
%         rotation=75,%
%         densityx=2,%
%         densityy=7,%
%         densityz=2%
%     }
% \end{tikzpicture}

% \end{document}

% \resizebox{\textwidth}{!}{
\begin{tikzpicture}[node distance=0em, auto]

\tikzset{>=latex}

\tikzcuboid{
        shiftx=0cm,%
        shifty=0cm,%
        scale=1.00,%
        rotation=0,%
        dimx=1,
        dimy=1,
        dimz=1,
        densityx=8,%
        densityy=8,%
        densityz=8%
    };

% \node (tsne) {\includegraphics[height=5cm,trim={0 0 0 0},clip]{teaser/tsne.pdf}}; %images go here

% \node [right=0em of tsne] (recon) {\includegraphics[height=5cm,trim={0 0 0 0},clip]{teaser/teaser_reconstruct.pdf}}; %images go here

% \node [left=0em of tsne] (part) {\includegraphics[height=5cm,trim={0 0 0 0},clip]{teaser/training_part.pdf}}; %images go here

% \node [below=0em of part] (cap0) {(a) Training parts from ShapeNet.};
% \node [below=0em of tsne, align=left, shift={(1.5em, 0)}] (cap1) {(b) t-SNE plot of part embeddings.};
% \node [below=0em of recon, align=left] (cap2) {(c) Reconstructing entire scenes with Local Implicit Grids};
% \draw [color=gray, ->] (5, -0.6) -- (1, -0.3);
\end{tikzpicture}
% }
